# Supplementary material for: TRIDEnT: Building Decentralized Incentives for Collaborative Security
Source: arXiv:1905.03571 source file (2019-05-09)
Supplement: Supplementary file 1 [file appendix.tex]

\section{Cryptographic extensions}
\par\noindent\textbf{The problem of multicast equivocation: }
One requirement of the system is to be able to guarantee that the streams are
provided ``as advertised'', without differences among the different streaming instances.
In other words, we need an authentication and non-equivocation mechanism for distributed streaming.
This need cannot be satisfied by traditional streaming authentication schemes (e.g.~\cite{perrig2000efficient,perrig2002spins}),
as in our case the sender cannot be fully trusted, and, whereas the participants do not have very strict computational
restrictions when they run computations locally, computations performed on the ledger and data stored on it are much more expensive.
Therefore, we propose a construction for efficiently detecting and penalizing equivocation in data streaming.
We present our construction in Protocol~\ref{pr:stream}, with proofs of security to be included in the full version of the paper.
\begin{figure*}[h]
	\centering
	\fbox{\procedure{Non-equivocation protocol $NE$}{
		\textbf{Alice} \< \< \textbf{Contract} \< \< \textbf{Bob} \< \< \textbf{Charlie} \\
		%\qquad \< \< Hello give me some space\qquad \< \< Me too please a little bit more \< \< \qquad \\
		%\text{start $S$} \< \< \text{test12345 } \< \< \text{Hello test message} \< \< \< \\
		\< \sendmessagerightx[2cm]{0}{\text{deposit $D$, advertise $S$}} \< \< \< \< \< \\
		\> \< \< \< \sendmessageleft{length=2,top=start streaming} \> \< \< \> \\
		\> \sendmessagerightx[8.5cm]{8}{sign(0, H(s_0))} \< \< \<\\
		\> \sendmessagerightx[8.5cm]{8}{sign(1, H(s_0|s_1))} \< \< \<\\
		\> \< \< \> \< \< \sendmessagerightx[2cm]{2}{sign(0, H(s_0))} \> \<\\
		\< \< \< \ldots \ldots \< \< \<\\
		\> \sendmessagerightx[8.5cm]{8}{sign(m, H(\ldots|s_m))} \< \< \<\\
		\> \sendmessageleftx[8.5cm]{8}{\text{A long message for Alice}} \< \< \<\\
		%\text{last thing} \< \< \< \< \< \<
	}}
		\caption{Distributed streaming non-equivocation protocol}
		\label{pr:stream}
	\end{figure*}
In summary, the protocol works as follows.
\begin{enumerate}
	\item Before being able to advertise a stream, the stream producer (Alice), deposits an amount $\$D$ of tokens to a blockchain address
as collateral.
        \item Afterwards, Bob (a streamer) sees the posted advert and starts streaming. Alice authenticates the stream to Bob by
signing batches of data of size $k$ with her known public key.
        \item When another streamer Charlie wants to join the stream, Alice starts authenticating batches by using the same
key.
        \item At any point, a streaming party can issue a challenge of the form $sign(i, H(\cdots|s_i))$ to the blockchain. This challenge acts like a bounty on the streamer. If some
other streamer notices an inconsistency in his stream, then he can submit the authenticated message signed by Alice, to the ledger, as proof of misbehaviour.
        \item If misbehaviour is proven, the two streamers share the deposit, with the first party getting a larger share of the reward, and the stream is closed.
	\item In the scenario where Alice is honest, she can claim back the deposit after $T_1$ time steps have elapsed after she takes down the stream advertisement. Therefore, she cannot abort the
protocol instantly, in case she gets nervous by a challenge submitted.
\end{enumerate}
It is evident that this protocol scales very well with an increased
number of streamers. Actually, the effort by the streamers to guarantee the same level of security, is inversely proportional to the
number of (honest) streamers subscribed to a stream at any given time.
